# Supplementary material for: Separation of Artifacts from Spin-Torque Ferromagnetic Resonance Measurements of Spin-Orbit Torque for the Low-Symmetry van der Waals Semi-Metal ZrTe$_\textbf{3}$
Source: arXiv:2110.01720 source file (2021-12-05)
Supplement: Supplementary file 2 [file Supp_old.pdf]

Supporting Information for:

Separation of Artifacts from Spin-Torque Ferromagnetic  
Resonance Measurements of Spin-Orbit Torque for the  
Low-Symmetry van der Waals Semi-Metal  $\text{ZrTe}_3$

*Thow Min Cham,<sup>1</sup> Saba Karimeddiny,<sup>1</sup> Vishakha Gupta,<sup>1</sup> Joseph A. Mittelstaedt,<sup>1</sup>  
and Daniel C. Ralph<sup>1,2</sup>*

<sup>1</sup>Cornell University, Ithaca, NY 14850, USA

<sup>2</sup>Kavli Institute at Cornell, Ithaca, NY 14853, USA

**Contents**

|          |                                                                                |          |
|----------|--------------------------------------------------------------------------------|----------|
| <b>1</b> | <b>Estimate of the spin-pumping voltage</b>                                    | <b>2</b> |
| <b>2</b> | <b>Hall-ST-FMR calculation of <math>E_{\text{art}}</math></b>                  | <b>3</b> |
| <b>3</b> | <b><math>\text{ZrTe}_3</math> resistivity from resistance vs thickness fit</b> | <b>4</b> |
| <b>4</b> | <b>Raman Spectroscopy</b>                                                      | <b>6</b> |
| <b>5</b> | <b>Device dimensions</b>                                                       | <b>7</b> |

# 1 Estimate of the spin-pumping voltage

Here we estimate amplitude of the artifact voltage generated by spin-pumping together with the inverse spin Hall effect in our devices:<sup>[1-4]</sup>

$$S_{XX}^{\text{art, est}} = V_{\text{sp}} = -\frac{eB_0R_{\text{tot}}\xi_{\text{SH}}}{2\pi\alpha^2\gamma(2B_0 + \mu_0M_{\text{eff}})^2}g_{\text{eff}}^{\uparrow\downarrow}\lambda_{\text{sd}}\tanh\left(\frac{t_{\text{ZrTe}}}{2\lambda_{\text{sd}}}\right) \times [(\tau_{\parallel}^0)^2 + (1 + \frac{\mu_0M_{\text{eff}}}{B_0})(\tau_{\perp}^0)^2] \times S(B)\cos^2\phi \begin{cases} L \sin \phi & \text{longitudinal} \\ W \cos \phi & \text{transverse} \end{cases} \quad (1)$$

Here  $R_{\text{tot}}$  is the device resistance,  $g_{\text{eff}}^{\uparrow\downarrow}$  is the effective spin mixing conductance and  $\lambda_{\text{sd}}$  is the spin diffusion length in the ZrTe<sub>3</sub>. In our estimate we use values for  $B_0$ ,  $M_{\text{eff}}$ ,  $\alpha$ ,  $\tau_{\parallel}^0$ ,  $\tau_{\perp}^0$  and  $\xi_{\text{SH}}$  determined from the Hall ST-FMR measurements,  $R_{\text{tot}}$  from 2-point resistance measurements, and  $t_{\text{ZrTe}}$  from atomic force microscopy. We assume a spin-mixing conductance of  $g_{\text{eff}}^{\uparrow\downarrow} \approx 2 \times 10^{19} \text{ m}^{-2}$  as measured for Pt/Py bilayers<sup>[3]</sup> and a spin diffusion length of  $\lambda_{\text{sd}} \approx 1 \text{ nm}$  which is typical for strong spin-orbit materials.<sup>[5,6]</sup> **Supplementary Figure 1** shows that the estimated artifact voltage  $S_{XX}^{\text{art, est}}$  has the same order of magnitude as the measured signal  $S_{XX}^{\text{AMR}}$  for ZrTe<sub>3</sub> layers thicker than about 10 nm. This agrees with our conclusions in the main text based on the Hall-detected ST-FMR measurements that the standard ST-FMR analysis is dominated by artifacts in this thickness range, and indicates that spin pumping is a major contributor to the artifact voltage. Given uncertainties in the values of  $g_{\text{eff}}^{\uparrow\downarrow}$  and  $\lambda_{\text{sd}}$ , the Hall analysis presented in the main text (Fig. 8(a)) gives more precise measurements of the artifact voltages.

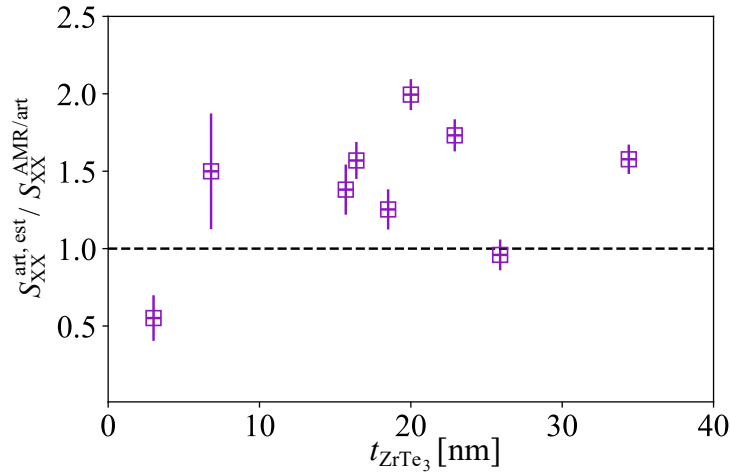

Figure 1: Estimated ratio of spin pumping artifact  $S_{XX}^{\text{art, est}}$  to the measured symmetric ST-FMR signal  $S_{XX}^{\text{AMR/art}}$  for the longitudinal ST-FMR geometry. The error bars plotted do not include uncertainties in the parameters  $g_{\text{eff}}^{\uparrow\downarrow}$  and  $\lambda_{\text{sd}}$ .

## 2 Hall-ST-FMR calculation of $E_{\text{art}}$

The artifact voltage due to spin-pumping can be quantified from the symmetric and antisymmetric resonance amplitudes from the AHE and PHE Hall readouts in addition to the conventional AMR readout. Using Equations (11) and (12) in the main text <sup>[4]</sup>

$$\frac{-A_{\text{XY}}^{\text{AHE}}}{S_{\text{XY}}^{\text{AHE}/\text{art}} + W(E_{\text{art}}/2)} = \frac{S_{\text{XY}}^{\text{PHE}/\text{art}} + W(E_{\text{art}}/2)}{A_{\text{XY}}^{\text{PHE}}} \quad (2)$$

$$\frac{-A_{\text{XY}}^{\text{AHE}}}{S_{\text{XY}}^{\text{AHE}/\text{art}} + W(E_{\text{art}}/2)} = \frac{S_{\text{XX}}^{\text{AMR}/\text{art}} + L(E_{\text{art}}/2)}{A_{\text{XX}}^{\text{AMR}}} \quad (3)$$

we obtain two independent formulas for  $E_{\text{art}}$ . From Eq. (2):

$$E_{\text{AHE, PHE}}^{\pm/\text{art}} = -\frac{(S_{\text{XY}}^{\text{AHE}/\text{art}} + S_{\text{XY}}^{\text{PHE}/\text{art}})}{W} \pm \frac{\sqrt{(S_{\text{XY}}^{\text{AHE}/\text{art}} + S_{\text{XY}}^{\text{PHE}/\text{art}})^2 - 4(S_{\text{XY}}^{\text{AHE}/\text{art}} S_{\text{XY}}^{\text{PHE}/\text{art}} + A_{\text{XY}}^{\text{AHE}} A_{\text{XY}}^{\text{PHE}})}}{W} \quad (4)$$

and from Eq. (3):

$$E_{\text{AHE, AMR}}^{\pm/\text{art}} = -\frac{(S_{\text{XY}}^{\text{AHE}/\text{art}} L + S_{\text{XX}}^{\text{AMR}/\text{art}} W)}{WL} \pm \frac{\sqrt{(S_{\text{XY}}^{\text{AHE}/\text{art}} L + S_{\text{XX}}^{\text{AMR}/\text{art}} W)^2 - 4WL(S_{\text{XY}}^{\text{AHE}/\text{art}} S_{\text{XX}}^{\text{AMR}/\text{art}} + A_{\text{XY}}^{\text{AHE}} A_{\text{XX}}^{\text{AMR}})}}{WL} \quad (5)$$

Values calculated using either the "+" or "-" sign in Equation (4) can be checked against "+" or "-" values from Equation (5) for consistency. We find that values calculated using  $E_{\text{AHE, PHE}}^{+/\text{art}}$  and  $E_{\text{AHE, AMR}}^{+/\text{art}}$  are consistent. In contrast, the  $E_{\text{AHE, PHE}}^{-/\text{art}}$  values gave an unphysical change in sign even for the thinnest  $\text{ZrTe}_3$  device (**Supplementary Figure 2**).

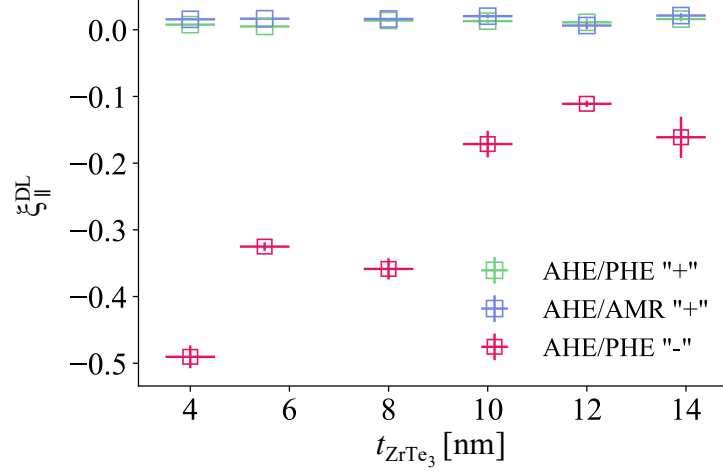

Figure 2: Comparison of corrected  $\xi_{||}^{\text{DL}}$  values calculated using  $E_{\text{AHE,PHE}}^{\pm/\text{art}}$ .

### 3 ZrTe<sub>3</sub> resistivity from resistance vs thickness fit

Assuming that the resistivity of ZrTe<sub>3</sub> remains approximately constant with thickness, we can estimate the resistivity of the Permalloy and ZrTe<sub>3</sub> layers in our heterostructure using a parallel resistor model

$$\frac{1}{R_{\text{device}}} = \frac{W}{L\rho_{\text{ZrTe}_3}}t_{\text{ZrTe}_3} + \frac{W}{L\rho_{\text{Py}}}t_{\text{mag}} \quad (6)$$

where  $t_{\text{ZrTe}_3}$  is the ZrTe<sub>3</sub> thickness as measured by atomic force microscopy,  $t_{\text{mag}}$  is the thickness of the permalloy layer, and  $L$  and  $W$  are the device lengths and widths respectively. From a linear fit to  $L/(WR)$  vs  $t_{\text{ZrTe}_3}$  (**Supplementary Figure 3a**) we calculate  $\rho_{\text{ZrTe}_3} = 570 \pm 70 \mu\Omega\text{cm}$ , in agreement with values previously reported.<sup>[7]</sup> We also obtain  $\rho_{\text{Py}} = 90 \pm 10 \mu\Omega\text{cm}$ , similar to previous values reported in our group for glancing angle sputtered Py.<sup>[8,9]</sup> We calculate the Oersted field contribution to the field-like spin conductivity (Supplementary Figure 3b) using the equation  $\sigma_{\text{Oe}} = \frac{e}{\hbar}\mu_0 M_{\text{eff}} t_{\text{mag}} t_{\text{ZrTe}_3} \sigma_{\text{ZrTe}_3}$ , where  $\sigma_{\text{ZrTe}_3} = 1/\rho_{\text{ZrTe}_3}$ . The uncertainty in the Oersted torque values was estimated from the linear fits for  $\rho_{\text{ZrTe}_3}$ .

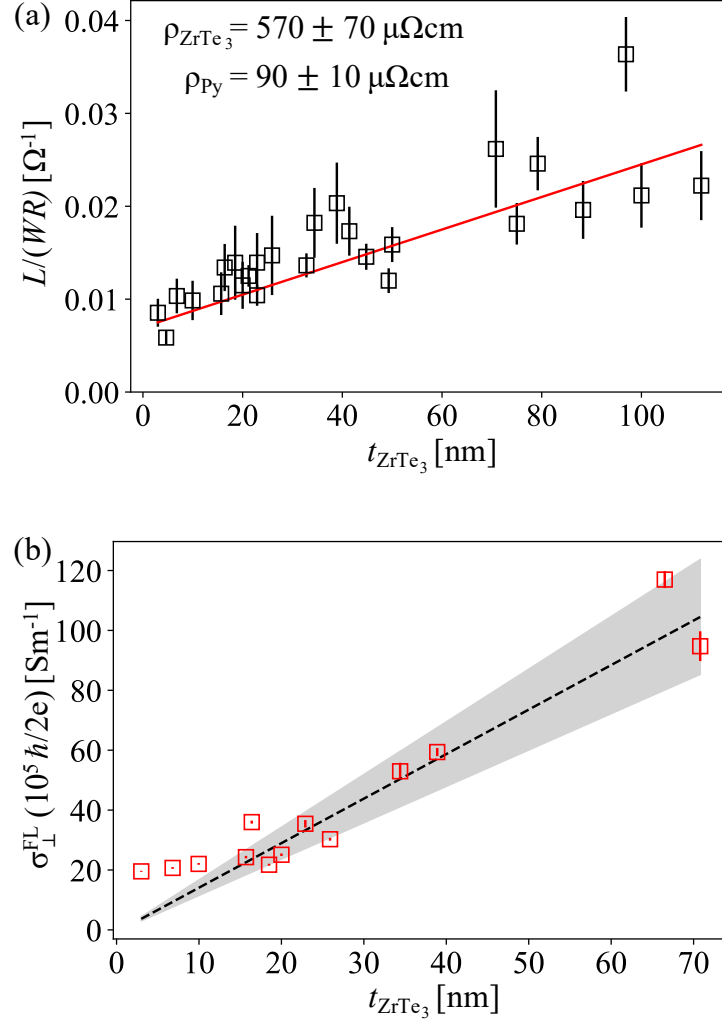

Figure 3: (a) Linear fit of the device-geometry-normalized conductance  $L/(WR)$  versus the thickness of the  $\text{ZrTe}_3$  layer. (b) Field-like spin conductivity as a function of  $\text{ZrTe}_3$  thickness from current-calibrated STFMR measurements. The Oersted torque (gray shaded region) accounts quantitatively for the field-like torques for  $\text{ZrTe}_3$  thicker than  $\approx 15$  nm.

## 4 Raman Spectroscopy

We perform polarized Raman spectroscopy on the fabricated devices and confirm that the  $\text{ZrTe}_3$  layer retains its as-grown characteristics after the nano-fabrication processes. We use a 532 nm excitation laser on a Witec Alpha 300R confocal Raman microscope with a rotation stage and observe three main peaks at 108, 145 and 213  $\text{cm}^{-1}$ , in agreement with space group  $P2_1/m$  as previously reported in the literature.<sup>[7,10]</sup>

The relative amplitudes of the peaks change as the angle between the polarization direction and the crystal axis is changed. **Supplementary Figure 4a,b** shows the decrease in the amplitude of the peak at 213  $\text{cm}^{-1}$  as the angle  $\phi$  between the laser polarisation and device current axis is swept from  $0^\circ$  to  $90^\circ$ . We use this to confirm that the devices were fabricated so that the applied current flows along the b axis perpendicular to the mirror plane of  $\text{ZrTe}_3$ .

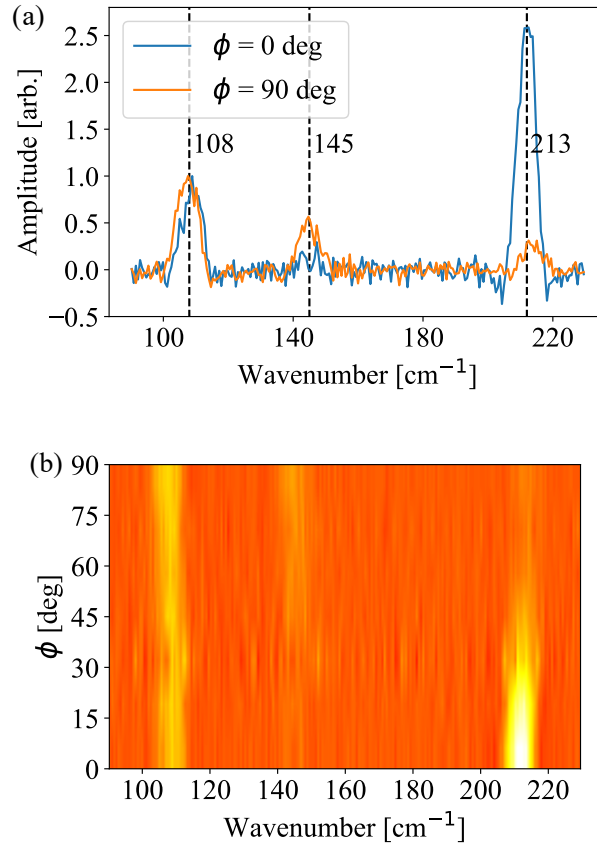

Figure 4: Polarized Raman spectroscopy of a  $\text{ZrTe}_3$  device used to confirm the crystal quality and crystal-axis direction, where  $\phi$  is the angle between the laser polarisation ( $E$ ) and the device current axis ( $I$ ). (a) Comparison between spectra for  $\phi = 0^\circ$  ( $E \parallel I$ ) and  $\phi = 90^\circ$  ( $E \perp I$ ). (b) Colormap of the spectra evolution as a function of the angle between the polarization and current directions. The Raman peak at 213  $\text{cm}^{-1}$  decreases as the polarization angle is rotated from  $0^\circ$  to  $90^\circ$ .

## 5 Device dimensions

| Device | Type       | Thickness [ $\mu\text{m}$ ] | Length [ $\mu\text{m}$ ] | Width [ $\mu\text{m}$ ] | Resistance [ $\Omega$ ] |
|--------|------------|-----------------------------|--------------------------|-------------------------|-------------------------|
| 1      | STFMR      | 3                           | 3                        | 3                       | 118                     |
| 2      | STFMR      | 4.66                        | 4                        | 3                       | 230                     |
| 3      | STFMR      | 6.8                         | 3                        | 3                       | 97                      |
| 4      | STFMR      | 9.96                        | 3                        | 3                       | 81                      |
| 5      | STFMR      | 15.7                        | 2.5                      | 2.5                     | 92                      |
| 6      | STFMR      | 16.4                        | 3                        | 3                       | 75                      |
| 7      | STFMR      | 18.5                        | 2                        | 2                       | 80                      |
| 8      | STFMR      | 20                          | 2.5                      | 2.5                     | 87.3                    |
| 9      | STFMR      | 22.9                        | 2.5                      | 2.5                     | 72                      |
| 10     | STFMR      | 25.9                        | 2                        | 2                       | 66                      |
| 11     | STFMR      | 34.4                        | 3                        | 3                       | 55                      |
| 12     | STFMR      | 38.9                        | 3                        | 3                       | 50                      |
| 13     | STFMR      | 57.1                        | 13                       | 5                       | 72                      |
| 14     | STFMR      | 66.5                        | 13                       | 4                       | 72                      |
| 15     | STFMR      | 70.8                        | 3                        | 3                       | 37.2                    |
| 16     | Hall STFMR | 4                           | 4                        | 2.2                     | 365                     |
| 17     | Hall STFMR | 5.5                         | 5                        | 3                       | 221                     |
| 18     | Hall STFMR | 6.5                         | 4                        | 2.5                     | 250                     |
| 19     | Hall STFMR | 8                           | 6                        | 3                       | 200                     |
| 20     | Hall STFMR | 10                          | 5                        | 4                       | 39                      |
| 21     | Hall STFMR | 12                          | 4                        | 2                       | 250                     |
| 22     | Hall STFMR | 13.9                        | 5.5                      | 3.5                     | 180                     |
| 23     | Hall STFMR | 21.2                        | 6                        | 4                       | 120                     |
| 24     | Hall STFMR | 22.9                        | 5                        | 3                       | 160                     |
| 25     | Hall STFMR | 32.8                        | 6                        | 4                       | 110                     |
| 26     | Hall STFMR | 41.4                        | 4                        | 3                       | 77                      |
| 27     | Hall STFMR | 44.8                        | 6                        | 4                       | 103                     |
| 28     | Hall STFMR | 49.3                        | 5                        | 3                       | 139                     |
| 29     | Hall STFMR | 50                          | 5                        | 3                       | 105                     |
| 30     | Hall STFMR | 75                          | 5                        | 3                       | 92                      |
| 31     | Hall STFMR | 79.2                        | 6                        | 4                       | 61                      |
| 32     | Hall STFMR | 88.3                        | 4                        | 3                       | 68                      |
| 33     | Hall STFMR | 96.9                        | 8                        | 4                       | 55                      |
| 34     | Hall STFMR | 100                         | 4                        | 3                       | 63                      |
| 35     | Hall STFMR | 112                         | 4                        | 3                       | 60                      |

## References

- [1] Y. Tserkovnyak, A. Brataas, G. E. W. Bauer, *Phys. Rev. Lett.* **2002**, 88, 117601.
- [2] Y. Tserkovnyak, A. Brataas, G. E. W. Bauer, *Phys. Rev. B* **2002**, 66, 224403.
- [3] O. Mosendz, V. Vlaminck, J. E. Pearson, F. Y. Fradin, G. E. W. Bauer, S. D. Bader, A. Hoffmann, *Phys. Rev. B* **2010**, 82, 214403.
- [4] S. Karimeddiny, J. A. Mittelstaedt, R. A. Buhrman, D. C. Ralph, *Phys. Rev. Applied* **2020**, 14, 024024.
- [5] J. C. R. Sánchez, L. Vila, G. Desfonds, S. Gambarelli, J. P. Attané, J. M. De Teresa, C. Magén, A. Fert, *Nature Communications* **2013**, 4, 2944.
- [6] A. R. Mellnik, J. S. Lee, A. Richardella, J. L. Grab, P. J. Mintun, M. H. Fischer, A. Vaezi, A. Manchon, E. A. Kim, N. Samarth, D. C. Ralph, *Nature* **2014**, 511, 449.
- [7] A. Geremew, M. A. Bloodgood, E. Aytan, B. W. K. Woo, S. R. Corber, G. Liu, K. Bozhilov, T. T. Salguero, S. Rumyantsev, M. P. Rao, A. A. Balandin, *IEEE Electron Device Lett.* **2018**, 39, 735.
- [8] M. H. Guimarães, G. M. Stiehl, D. MacNeill, N. D. Reynolds, D. C. Ralph, *Nano Lett.* **2018**, 18, 1311.
- [9] D. MacNeill, G. M. Stiehl, M. H. Guimaraes, R. A. Buhrman, J. Park, D. C. Ralph, *Nat. Phys.* **2017**, 13, 300.
- [10] S. Yang, H. Cai, B. Chen, C. Ko, V. O. Özçelik, D. F. Ogletree, C. E. White, Y. Shen, S. Tongay, *Nanoscale* **2017**, 9, 12288.
